# Supplementary material for: Tokenization Preference for Human and Machine Learning Model: An Annotation Study
Source: arXiv:2304.10813 source file (2024-02-16)
Supplement: Supplementary file 1 [file appendix.tex]

\section{Original UI Instruction in Japanese}
Figure \ref{fgr:ranking_ja} and Figure \ref{fgr:annotation_ja} show the UI instruction texts in Japanese that are originally used in the annotation for the ranking annotation (\S \ref{sec:ranking_anno}) and the BoW annotation (\S \ref{sec:speed_anno}), respectively.

\begin{figure*}[t]
\centering
\includegraphics[width=15cm]{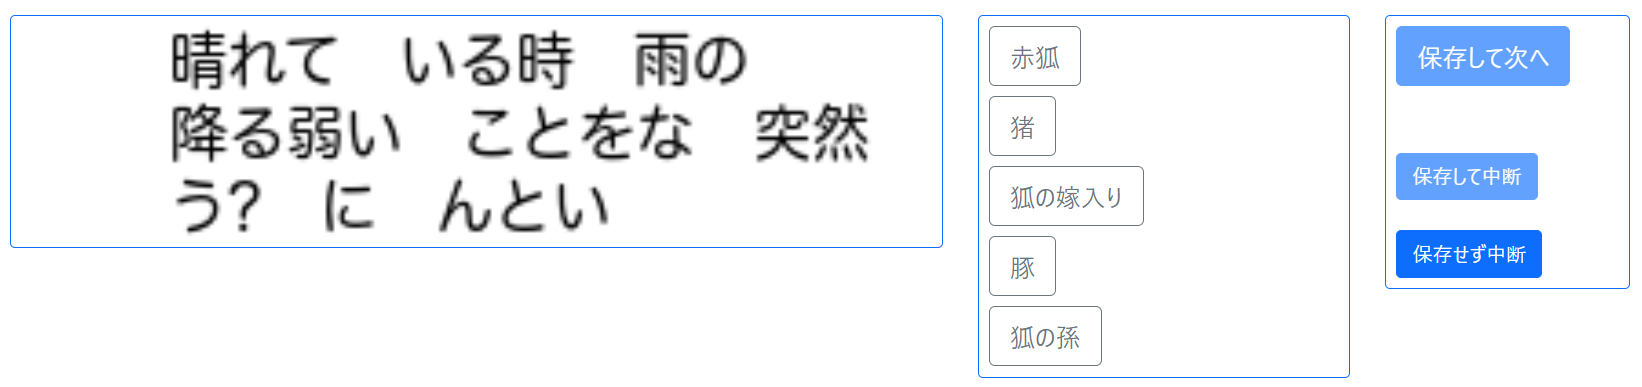}
\caption{
    Actually used UI instructions in Japanese for the QA annotation.
}
\label{fgr:annotation_ja}
\end{figure*}

\begin{figure}[t]
\centering
\includegraphics[width=7.9cm]{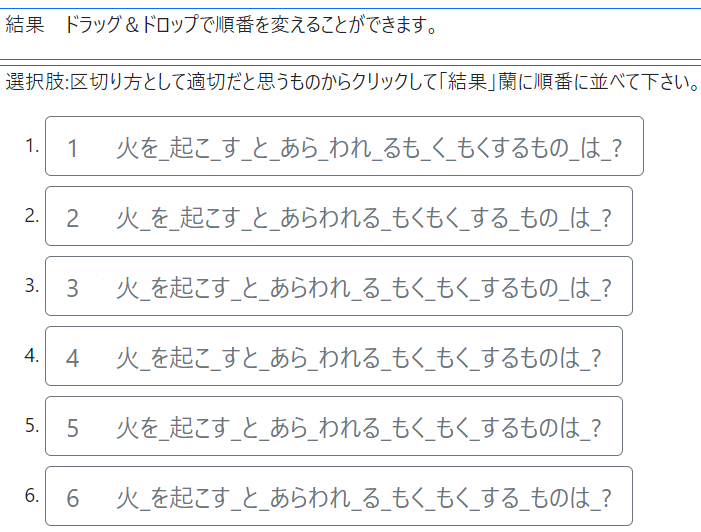}
\caption{
    Actually used UI in Japanese for the ranking annotation.
}
\label{fgr:ranking_ja}
\end{figure}

\section{QA Annotation with Vertical Style}
Additionally, to the human tractability annotation in \S \ref{sec:annotation}, we conducted an experiment in the setting where tokenized questions are shown vertically (Figure \ref{fgr:column}).
Because tokens are shown in an original order different from the BoW setting, native Japanese speakers can easily reproduce the original meaning.
We expect that this display style makes the effect of tokenization difference small.
Table \ref{tbl:column_result} summarizes the annotation result in this style.
The obtained tendency is different from Table \ref{tbl:result} because the result is affected by factors that we did not considered (e.g., the first characters in each token).

\label{sec:column_qa}
\begin{figure*}[t]
\centering
\includegraphics[width=15cm]{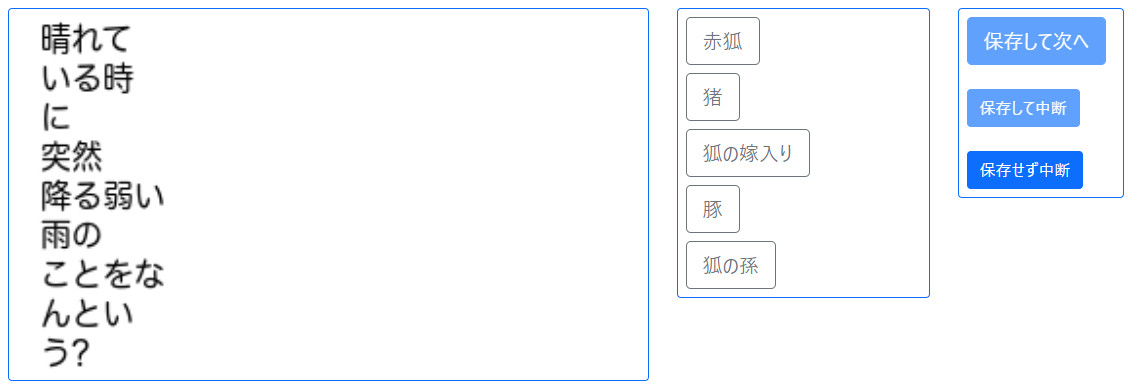}
\caption{
    UI instructions in Japanese for the QA annotation with vertical style tokenization.
}
\label{fgr:column}
\end{figure*}

\begin{table*}[ht]
\centering
\begin{tabular}{lrrrrrr}
\hline
                 & MeCab & Unigram  & BPE   & MaxMatch & OpTok  & Random        \\ \hline
\textit{Accuracy of Human (\%)} &   &        &        &         &             &               \\
Train            & 94.71  & 94.76     & 94.77   & 94.87   & \b{94.93}    & \u{94.48}      \\
Valid            & 96.51  & \b{97.32}     & 96.87   & 96.96   & 96.78    & \u{96.34}           \\
Total            & 94.91  & 95.05     & 95.01   & 95.10   & \b{95.14}    & \u{94.69}  \\ \hline
\textit{Response Time (sec.)}     &                &                &                &                &             &               \\
Train            & 4.02  & 3.99     & 4.00   & \u{3.94}   & 3.97    & \b{4.09}    \\
Valid            & 2.89  & 2.91     & 2.91   & \b{2.98}   & \u{2.82}    & 2.96          \\
Total            & 3.89  & 3.86     & 3.88   & \u{3.83}   & 3.84    & \b{3.96}   \\ \hline
\end{tabular}
\caption{
    The performance of machiineML learning models and annotation results for the JCommonsenseQA dataset with six tokenization methods.
    The highest and lowest values in each raw are highlighted with bold and underline, respectively.
    %各トークン分割手法で問題文を区切って提示した際の，読みやすさ1位の割合（\%，学習データの3,302件）と正解率（\%），平均回答時間（単位は秒，正答・回答時間が30秒以内のサンプルのみを集計），各サンプルの問題文の平均トークン数．
    \label{tbl:column_result}
}
\end{table*}

\section{Inconsistency of Ranking Annotation}
\label{sec:inconsistency}
The ranking annotation was performed by a single annotator from the beginning to the end of the QA dataset (the final 1,119 samples correspond to the validation split).
As reported in \S \ref{sec:acc_vs_ranking}, the MeCab tokenization scored lower in the validation split but scored the highest overall.
We discovered the shift brings about this outcome in the standard for the appropriateness of tokenization through the annotation.
Figure \ref{fgr:history_of_first} shows the averaged ranking of MeCab, Unigram, and Random for every 100 samples.
The annotator tended to assign higher scores to Unigram after the 8,000th sample as shown in the figure above.
Because the validation split is created from the final 1,119 samples, ``Appropriateness'' in Table \ref{tbl:result} shows a different tendency.
Considering that the ranking of Random is consistently the lowest, the annotation itself is conducted seriously.
We have 17 questions that have the completely same question text appearing in both the training and validation splits.
Nine out of seventeen questions are assigned that MeCab tokenization is the most appropriate in the training split. However, in the validation split, 4 out of 9 questions are assigned that other tokenizations such as Unigram and BPE are the most appropriate.
This result shows that the standard of tokenization appropriateness was changed during the annotation work.

To eliminate the effect of the change in the annotation standard, we conducted the experiments again with the QA dataset whose training and validation splits were shuffled.
Table \ref{tbl:result_shuffle} shows the results corresponding to Table \ref{tbl:tokenizationInfo} and \ref{tbl:result}.
The result does not contradict the statement in \S \ref{sec:results}.

% validの特性について追記する！
% validがおかしい理由→trainingデータ、validデータの順にアノテーションを行った。アノテーションをすすめる中で、「適切」の解釈が変わっていた（Appendixの図、どんどんspが増えていく）。本実験では、「適切」さについてインストラクションを与えていないため、人間は「適切な分割」に対する解釈に一貫したアノテーションを行うことが難しい。そのため、このサブセクションでは、全体的な傾向として、totalでの順位で議論する。
% シャッフルした実験もやったおy。
% ValidとTrainの両方に出てくる質問（選択肢が異なる）も17件あるが、trainでmecabが1stだった質問9件のうち、4件がspやbpeに変わっていた

% 1人で全体を担当し、過去のアノテーション結果にもアクセスできる状態だったが、一貫性に書けるものになった。
% randomはちゃんと下位なので、適当にやったとは考えられない。

\begin{figure}[t]
\centering
\includegraphics[width=7.9cm]{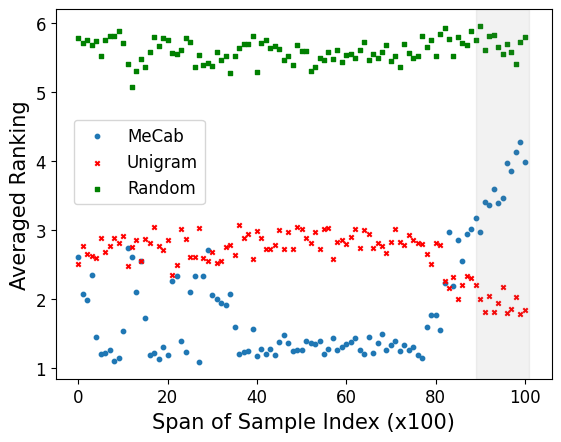}
\caption{
    Averaged ranking of MeCab, Unigram, and Random for every 100 samples.
    The annotation was conducted at the beginning of the data.
    The shaded part represents the validation splits.
}
\label{fgr:history_of_first}
\end{figure}

\begin{table*}[ht]
\centering
\begin{tabular}{lrrrrrr}
\hline
                               & MeCab      & Unigram & BPE        & MaxMatch   & OpTok  & Random         \\ \hline
\textit{Size of Vocabulary}    &            &         &            &            &        &                \\
Vocab of Tokenizer             & -          & 64,000  & 64,000     & 64,000     & 64,000 & -              \\
Vocab Used in Train            & 8,692      & 11,227  & 11,597     & 12,152     & 10,758 & 17,528      \\ 
Vocab Used in Valid            & 2,418      & 3,101   & 3,290      &  3,367     & 2,966  & 3,952          \\   
Vocab Used in Total            & 9,267      & 11,921  & 12,292     & 12,890     & 11,440 & 19,077         \\ \hline
\textit{Tokenization Length} &              &         &            &            &        &                \\
Train                          & 10.20      & 8.02    & 7.77       & \u{7.71}       & 8.39   & \b{10.56}         \\
Valid                          & 10.32      & 8.11    & 7.93       & \u{7.86}       & 8.49   & \b{10.68}       \\
Total                          & 10.21      & 8.03    & 7.79       & \u{7.73}  & 8.40   & \b{10.58}  \\ \hline
\textit{Entropy}               &            &         &            &            &        &                \\
Train                          & \u{8.27}   & 9.68    & 10.18      & 10.23      & 9.35   & \b{10.40}          \\
Valid                          & 8.91       & 9.08    & 9.52       & 9.56       & \u{8.80}   &\b{9.75}          \\
Total                          & \u{8.29} & 9.71    & 10.20      & 10.25      & 9.38   & \b{10.43} \\ \hline
\hline
\textit{Accuracy of Machine}    &                &                &       &          &                &               \\
Valid (Bag-of-Words)            & 39.92          & \b{41.91} & 40.75 & 41.41    & 41.29          & \u{39.29}   \\
Valid (BiLSTM)                  & 42.12          & 43.61          & 42.95 & 42.90    & \b{44.15} & \u{40.57}   \\ \hline
\textit{Appropriateness}        &                &                &       &          &                &               \\
Train                           & \u{1.86}     & 2.65           & 3.14  & 2.94     & 2.56           & \b{5.60} \\
Valid                           & \u{1.87}     & 2.67           & 3.13  & 2.98     & 2.50           & \b{5.61} \\
Total                           & \u{1.86}     & 2.65           & 3.14  & 2.95     & 2.55           & \b{5.61} \\ \hline
Accuracy of Human               &                &                &       &          &                &               \\
Train                           & \b{94.22} & 94.03          & 94.17 & 94.03    & 93.88          & \u{93.58}   \\
Valid                           & 95.08          & \b{95.97} & 95.17 & 94.72    & 95.53          & \u{94.45}   \\
Total                           & \b{94.30} & 94.25          & 94.28 & 94.11    & 94.06          & \u{93.67}   \\ \hline
\textit{Averaged Response Time} &                &                &       &          &                &               \\
Train                           & 5.44           & 5.37           & 5.44  & 5.42     & \u{5.35}     & \b{5.06} \\
Valid                           & 5.09           & \u{5.03}     & 5.07  & 5.17     & 5.05           & \b{5.98} \\
Total                           & 5.40           & 5.33           & 5.40  & 5.39     & \u{5.31}     & \b{6.05} \\ \hline
\end{tabular}
\caption{
    Tokenization information and experimental results on the newly created training/validation splits.
}
\label{tbl:result_shuffle}
\end{table*}

% annotation以外の情報をまとめる？
% perplexityとか、30秒以上かかったやつとか
% tokenizationの差は、table2とマージしてしまうと見やすいかも
